# Supplementary material for: Magnetic Order and Lattice Instabilities in Ni$_{2}$Mn$_{1+x}$Sn$_{1-x}$ Heusler based Magnetic Shape-Memory Alloys
Source: arXiv:1811.04221 source file (2018-11-10)
Supplement: Supplementary file 1 [file Supp.pdf]

## Supporting Information for

# Magnetic Order and Lattice Instabilities in $Ni_2Mn_{1+x}Sn_{1-x}$ Heusler based Magnetic Shape-Memory Alloys

Vijay Singh[1,2], Ambroise van Roekeghem[2], Swarup Kumar Panda[3,4], Subham Majumdar [1], Natalio Mingo[2] and Indra Dasgupta*[1, 3]

[1] Department of Solid State Physics, Indian Association for the Cultivation of Science, Jadavpur, Kolkata 700032, India

[2] CEA, LITEN, 17 Rue des Martyrs, 38054 Grenoble, France

[3] Centre for Advanced Materials, Indian Association for the Cultivation of Science, Jadavpur, Kolkata 700032, India

[4] Centre de Physique Theorique, Ecole Polytechnique, CNRS UMR 7644 Universite Paris-Saclay, 91128 Palaiseau, France

sspid@iacs.res.in.

**Figure S1**: The $L2_1$ cubic phase structure of the parent compound $Ni_2MnSn$ (a) and $Ni_2Mn_{1.5}Sn_{0.5}$ in both FM (b) and FI (c) phase, where Ni, Mn, $Mn_{Sn}$ and Sn are shown in blue, violet, green and gray color, respectively. The magnetic moments on the manganese are shown as arrows.

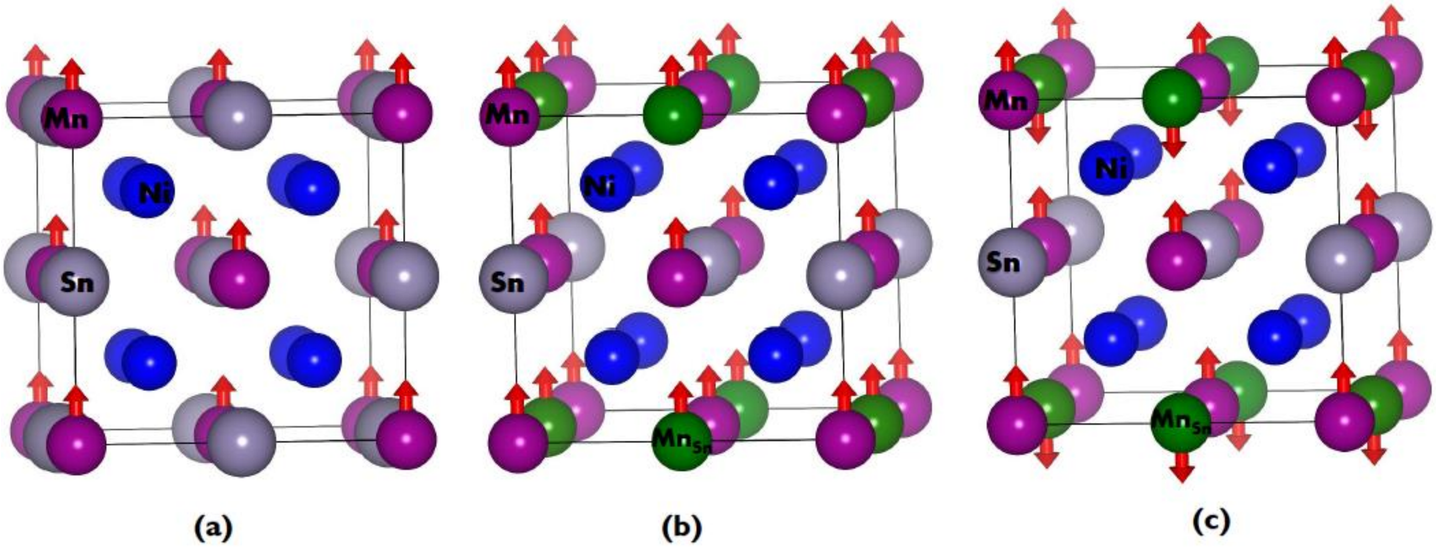

Figure S2: Full phonon dispersion of the ferromagnetic (a) $Ni_2MnGa$, and (b)$Ni_2MnSn$ along the Γ-X direction of the FCC BZ. The wave vector coordinate is in units of (2π/a).

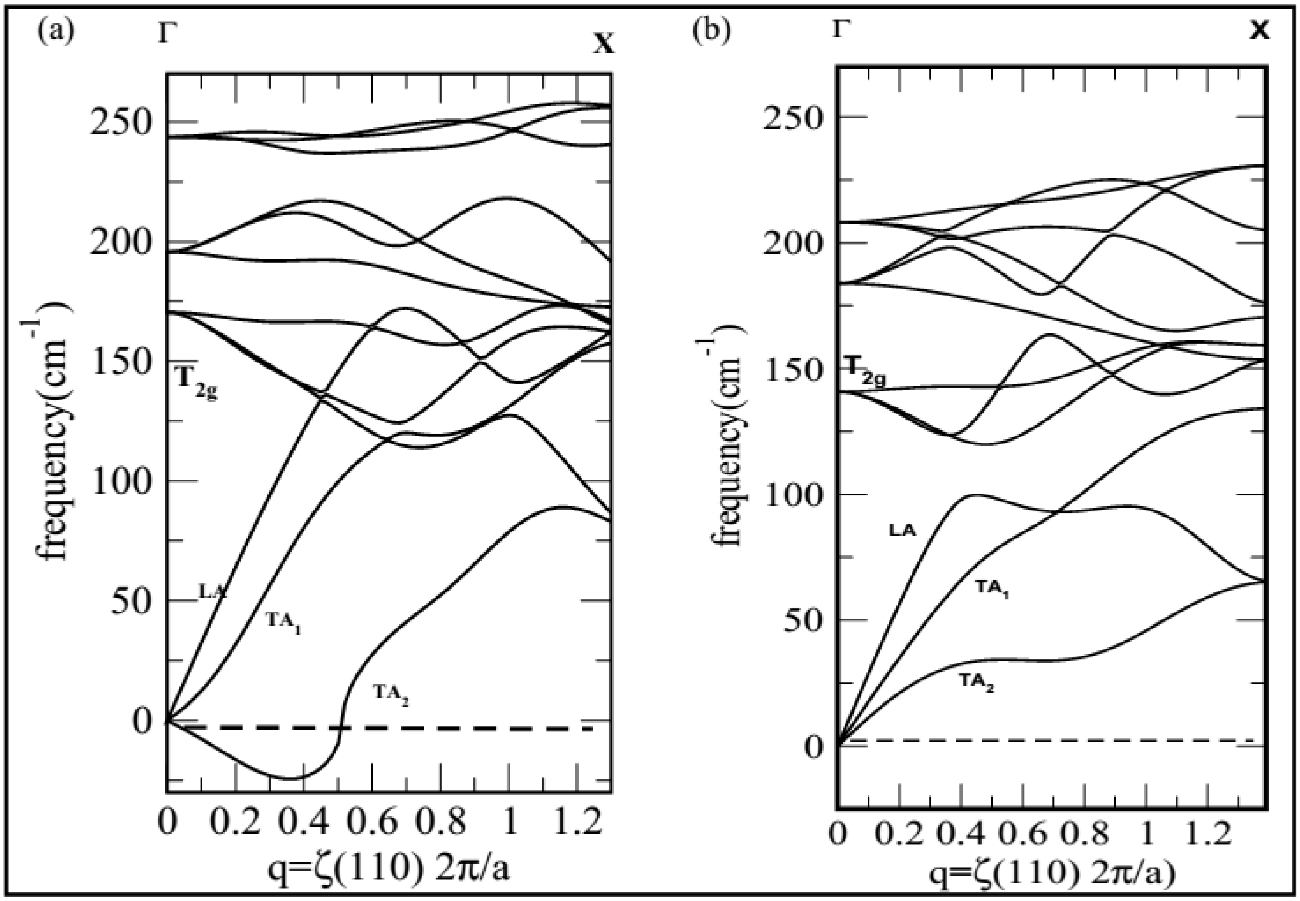

**Figure S3:** Full phonon dispersion along the high-symmetry lines of the BZ for both the FM and FI states of $Ni_2Mn_{1.5}Sn_{0.5}$ alloy using GGA method; here, we have adopted linear response DFPT formalism. The wave vector coordinate is in units of $(2\pi/a)$.

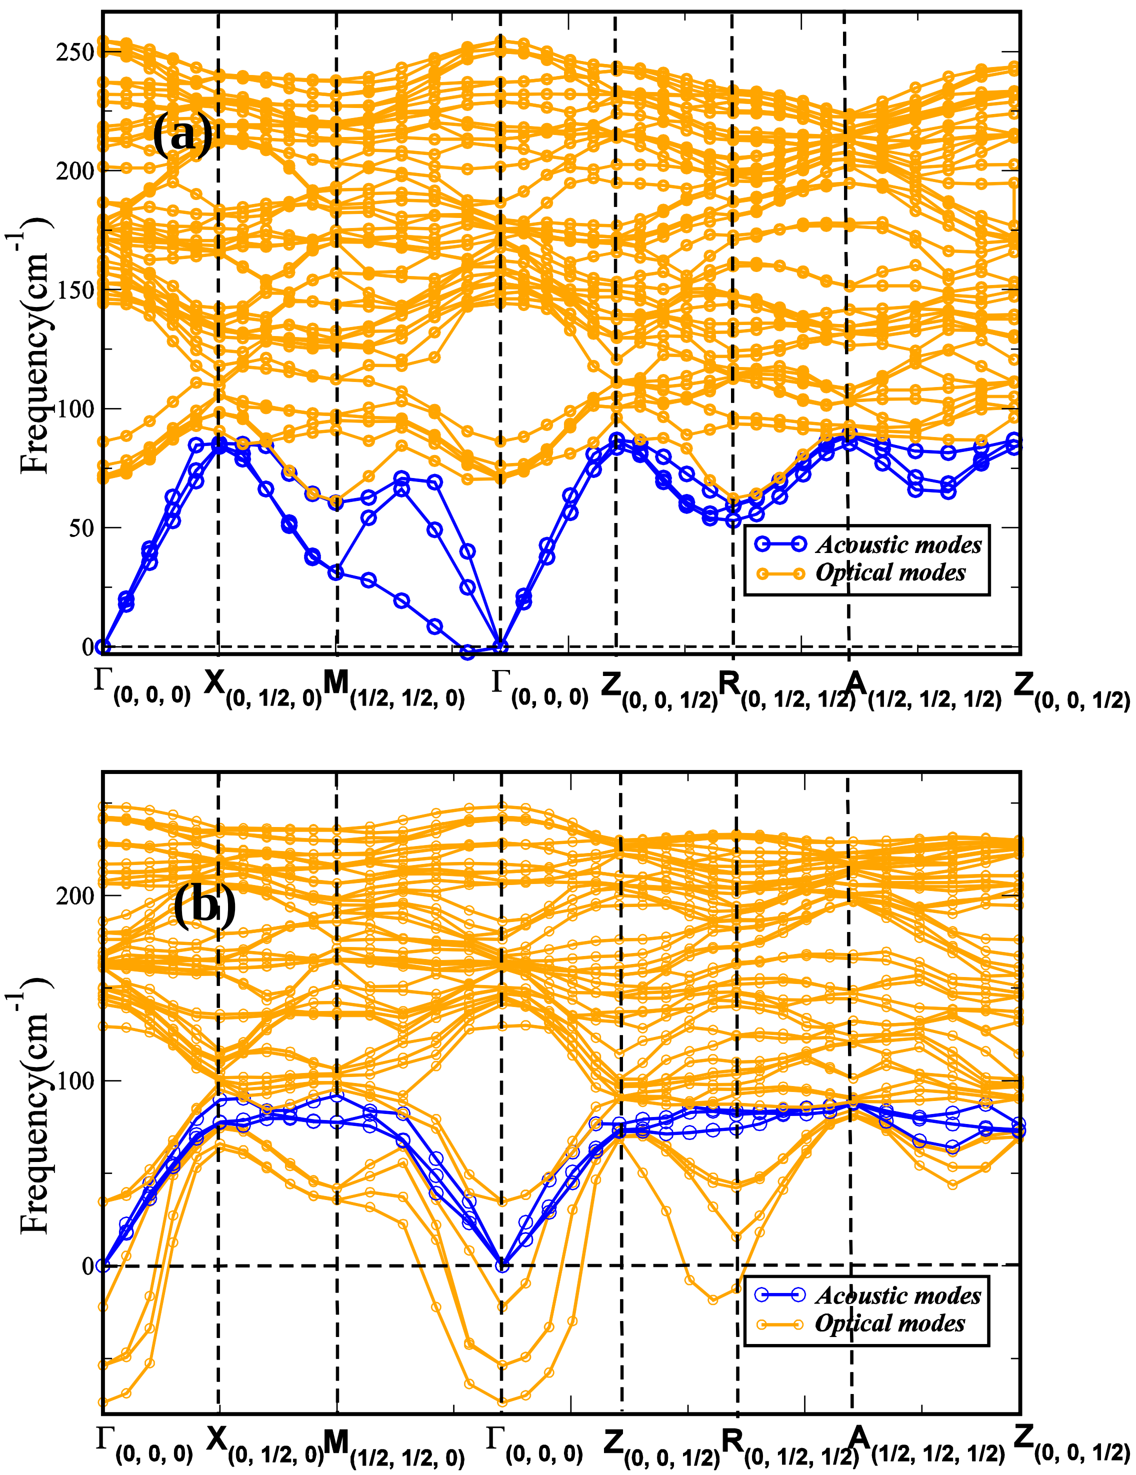

**Figure S4:** Cross-sections of the majority (left panel in blue) and minority-spin (right panel in green) Fermi surface for $Ni_2MnSn$ (a, b), $Ni_2Mn_{1.5}Sn_{0.5}$ in both (FM) (c, d) and (FI) (e, f) phase.

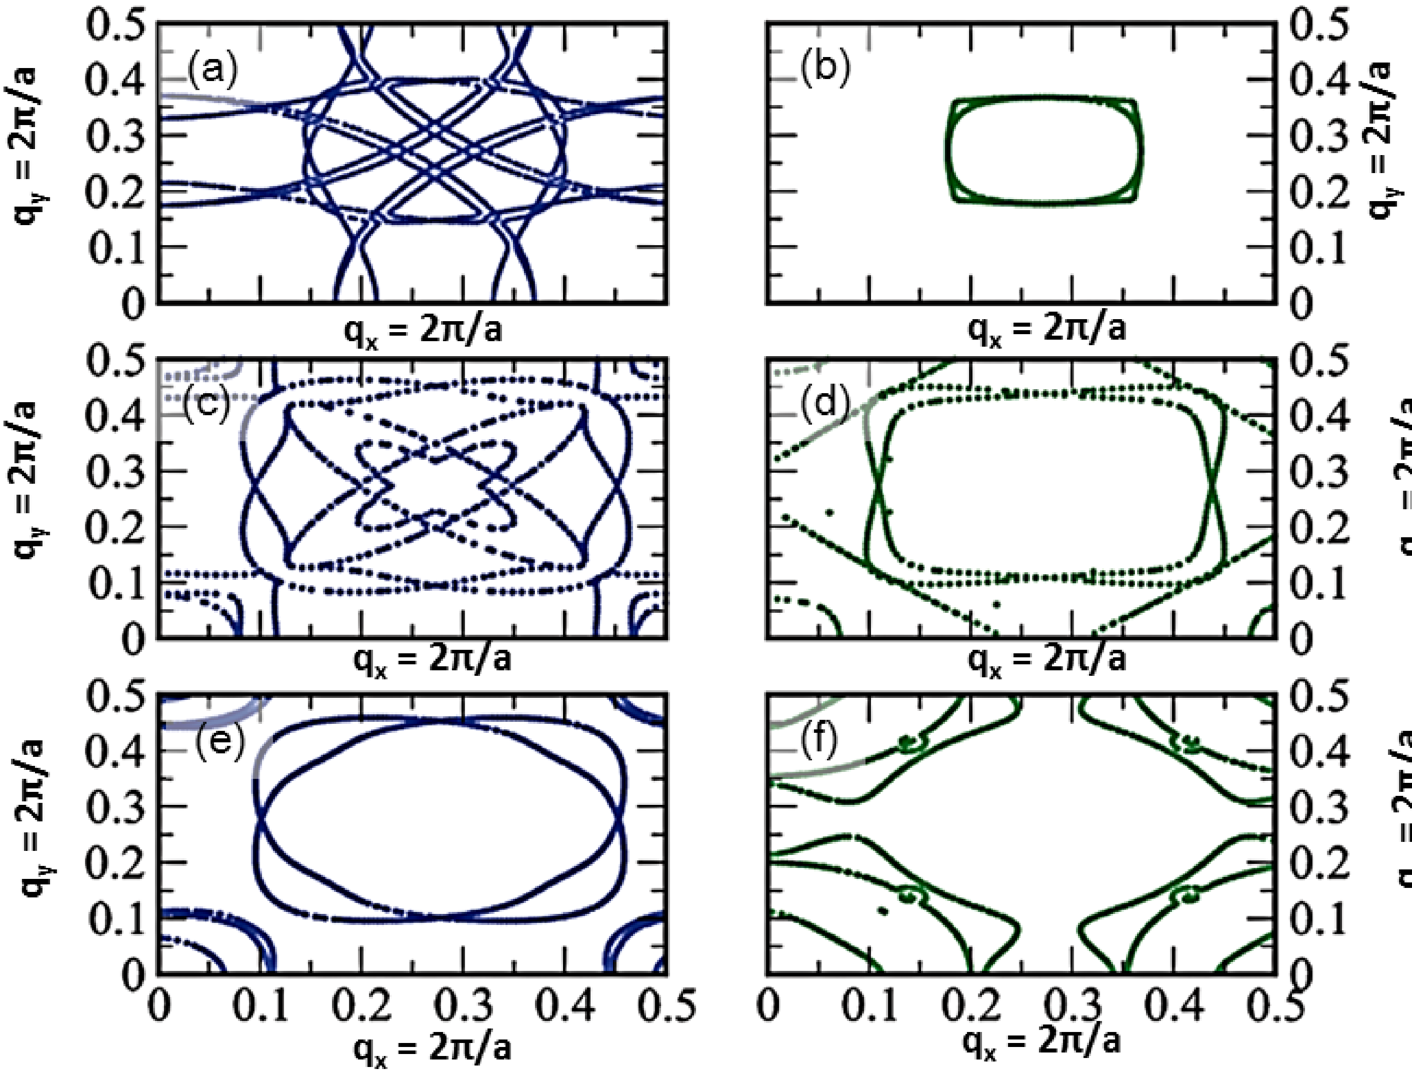

**Figure S5:** Full phonon dispersion of $Ni_2Mn_{1.5}Sn_{0.5}$ along the high-symmetry lines of the BZ for both FM (a) and FI (b) states obtained using PBE functional at 300° K . The wave vector coordinate is in units of $(2\pi/a)$. However, the stability of $Ni_2Mn_{1.5}Sn_{0.5}$ is observed at high temperature i.e. at 300° K for the FM states only.

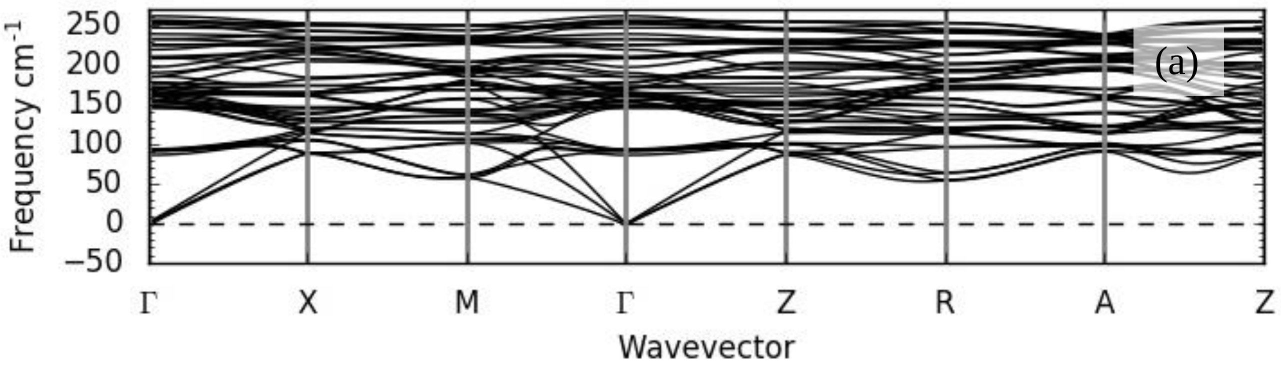


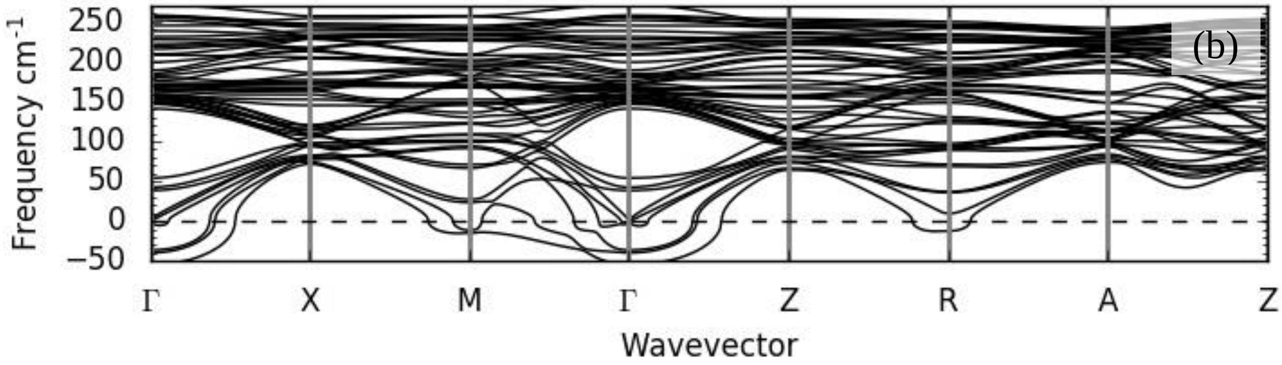

TABLE S2: Total magnetic moment, Lattice constant and Bond distances for both FM and FI states with and without relaxation in the $Ni_2Mn_{1.5}Sn_{0.5}$ alloy.

| Bond | Bond Length (Å) | | | |
|---|---|---|---|---|
| | Unrelaxed | | Relaxed | |
| | FM | FI | FM | FI |
| Lattice Constant (Å) | 5.99 | 5.99 | 5.968 | 5.955 |
| Total Mag. Mom. ($\mu_B$/f.u.) | 6.51 | 1.96 | 6.41 | 1.90 |
| Ni-Mn | 2.59 | 2.59 | 2.53 | 2.54 |
| Ni-$Mn_{Sn}$ | 2.59 | 2.59 | 2.53 | 2.54 |
| Ni-Sn | 2.59 | 2.59 | 2.64 | 2.62 |
| Mn-Mn | 4.24 | 4.24 | 4.22 | 4.21 |
| Mn-$Mn_{Sn}$ | 3.00 | 3.00 | 2.98 | 2.98 |
| Sn-Mn | 3.00 | 3.00 | 2.98 | 2.98 |
| Sn-$Mn_{Sn}$ | 4.24 | 4.24 | 4.22 | 4.21 |

## Details of  Plane-Wave Self-Consistent Field (PWSCF) Calculations

The lattice dynamical properties were calculated using the density functional perturbation theory (DFPT) as implemented in the Plane-Wave Self-Consistent Field (PWSCF) code using plane wave basis and ultra-soft pseudopotentials. The lattice parameters and kinetic energy cut-off  for the PWSCF calculations  are listed in the following table.

| **Compounds** | **Lattice parameters (Å)** | **Kinetic energy cutoff** |
|---|---|---|
| $Ni_2MnGa$ | 5.825 | 170 Ry |
| $Ni_2MnSn$ | 6.053 | |
| $Ni_2Mn_{1.5}Sn_{0.5}$ | 5.990 | |
| | | |

## **Details about the finite temperature lattice dynamics calculations :**

To examine the role of magnetic interactions for the stability of austenite phase at finite temperature we have performed finite temperature lattice dynamics calculations. We have used our recently developed inhouse code, quantum self-consistent ab-initio lattice dynamics approach (QSCAILD). QSCAILD is based on the calculation of temperature dependent interatomic force constants using regression analysis of forces obtained from DFT coupled with a harmonic model of the quantum canonical ensemble. The calculations are done in an iterative way to achieve self-consistency of the phonon spectrum.

In practice, we start from 0 K phonon spectrum which is calculated using small displacement method. From the phonon frequencies and eigenvectors of the initial phonon spectrum, we compute the matrix $\Sigma\ (i\alpha, j\beta)$ using the $\Gamma$ point of a $2 \times 2 \times 2$ supercell (128 atoms). The matrix $\Sigma$ which is a quantum covariance for atoms $i, j$ and directions $\alpha, \beta,$ is given by the following expression:

$$\Sigma(i\alpha, j\beta) = \frac{\hbar}{2\sqrt{M_i M_j}} \sum_m \omega_m^{-1}(1 + 2n_B(\omega_m))\varepsilon_{mi\alpha}\,\varepsilon_{mj\beta}^* \qquad (1)$$

where M is the atomic mass of the atom, $\omega_m$, the phonon frequency of mode m, $\varepsilon_m$ the corresponding wavefunction and $n_B$ the Bose-Einstein distribution. This matrix was further utilized as a covariance matrix of a multidimensional Gaussian distribution to generate N random sets (N = 100 for this work) of atomic displacements $\{u_{i\alpha}^n\}$, with $i$ indexing each atom and direction in the supercell and n is a given random configuration.

The forces acting on each atom of the supercell generated by this set of “n” random displacements was obatined using VASP based on DFT. Finally these forces and displacements are used  to fit the second- and third-order force constants of

a model potential, using least-squares minimization. These force constants allow us to calculate a new phonon spectrum and we iterate the process described above until the convergence.

Additionally, for each cycle of the convergence, we calculate the external pressure, $P = (\frac{\partial E_p}{\partial V})_S + (\frac{\partial E_k}{\partial V})_{S}$. As seen from the above expression, there are two main contributions to external pressure, $P$. First, the potential energy contribution, $E_{p,}$ which was obtained using the mean of the external pressure obtained by DFT and second the kinetic energy contribution, $E_{k,}$ where we adopt the quasiharmonic approach. We update the lattice parameter for every cycle until the mean external pressure of unit cell becomes negligible. The detailed description of the above methodology has also been discussed in our reference.[1]"

References

1. van Roekeghem A, Carrete J, Mingo N. Anomalous thermal conductivity and suppression of negative thermal expansion in $ScF_3$ Phys Rev B 2016, 94(2): 020303.
